# Supplementary material for: Numerical approximation of singular Forward-Backward SDEs
Source: arXiv:2106.15496 source file (2021-06-29)
Supplement: Supplementary file 1 [file appendix.tex]

%!TEX main = root

\section{Appendix}

\subsection{Numerical test of other methods}

%On the 2-dim toy model:\\
%- first explain that it can be transformed to a one dimensional pde and a way to obtain correct solution is e.g. to
%use particle system (or pde)
%\\
%- but we work in dimension 2 (again pde could be used) and we try
\begin{itemize}
%\item Bender-Zhang (in fact from the springer brief) it fails
%Always with toy model describe above. In Chassageneux et al, we take $K=8000$ sample paths of time-discretised
%Brownian motion and $m=10$ total Picard iterations. And trunctation constant $R=10$.
%\begin{center}
%\begin{figure}[!h] 
%\centering
%\includegraphics[width=8cm]{bender_zhang.png}
%\caption{With parameters $p=e=0$, $T=1$} 
%\end{figure}
%\end{center}
%
%It is clear that we observe the oscillation in the numerical solution figure, which does not correspond to the correct solution that we use particle system simulation, thus the Bender-Zhang method doesn't work in our setting. 
\item deep learning -> it fails : graphe final loss and computed solution. Expected from the litterature (no proof when degenracy is there)
Inspired by the article of Han et al, we train a simplified neural network model to get the numerical solution of toy model. However, the method of Han assumes a regular terminal condition which is not our case. Some figures are given in the following for different values of $\sigma$.
\\
By the spirit of the deep BSDE method, we employ a stochastic optimizer to solve the following stochastic optimization problem.
\begin{align}
	\inf_{\mu^{\pi}_0\in\mathcal{N}^{\prime}_0,\phi^{\pi}_i\in\mathcal{N}_i}F(\mu^{\pi}_0,\phi^{\pi}_0,...,\phi^{\pi}_{N-1})= \mathbb{E}|g(X^{\pi}_T) -Y^{\pi}_T|^ 2
\end{align}
where $\mathcal{N}^{\prime}_0$ and $\mathcal{N}_i$  $(0\leq i\leq N - 1)$ are parametric function spaces generated by neural net- works. In the analysis below, we assume the general case where $\mathcal{N}^{\prime}_0$ is subset of measurable functions from $\mathbb{R}^{m}$ to $\mathbb{R}$.
\\
In other words, the problem could be written in
\begin{align}
	&\inf_{Y_0,\{Z_t\}_{0\leq t\leq T}}\mathbb{E}|g(X^{\pi}_T) -Y^{\pi}_T|^ 2 ,\\&\textrm{s.t } X_t = \int_0^{T}Y_t\ud t+ \int_0^{T}\sigma(T-t)\ud W_t \\& Y_t = Z_t\ud W_t
\end{align}

We observe that the loss decreases as the iteration increases.

%\begin{figure}[ht]
%\begin{minipage}{0.3\linewidth}
%%\centering  % redundant
%\includegraphics[width=\textwidth]{DLsigma1.png}
%\caption{$\sigma=1$}
%\label{fig:figure1}
%\end{minipage}%
%\hfill% not: "\hspace{0.5cm}"
%\begin{minipage}{0.3\linewidth}
%%\centering  % redundant
%\includegraphics[width=\textwidth]{DLsigma03.png}
%\caption{$\sigma=0.3$}
%\label{fig:figure2}
%\end{minipage}%
%\hfill% not: "\hspace{0.5cm}"
%\begin{minipage}{0.3\linewidth}
%%\centering  % redundant
%\includegraphics[width=\textwidth]{DLsigma001.png}
%\caption{$\sigma=0.01$}
%\label{fig:figure3}
%\end{minipage}
%\end{figure}

For the three above figures corresponding to different $\sigma$, the numerical solution obtained via deep learning method and the (correct) solution by using Bossy's algorithm is totally different. Thus the deep learning method is not valid and not of our interests.
\newpage

\item Menozzi-Delarue in 2 dimension ? for burgers in dim 1 it fails (theoretical computation show entropy condition is not satisfied in dimension 1 + simulation in dimension 1).
We have the following toy model:
\begin{align}
dP_t& = \sigma\ud W_{t}\\
dE_t &= (P_t-Y_t)dt\ud t\\
dY_t &=  Z_t \ud W_t
\end{align}
In this case, we have our toy model written in dimension 2 with $U_t = (P_t,E_t)$
\begin{align*}
	U_t = \left(\begin{array}{c}
		p_0\\
		e_0
	\end{array}\right) + \int_{0}^{t}\left(\begin{array}{c}
		0\\
		P_s-Y_s
	\end{array}\right)\ud t + \int_0^{t}\left(\begin{array}{ccc}
		\sigma & 0\\
		0 & 0
	\end{array}\right)\ud W_s
\end{align*}
\begin{align*}
		Y_t = \phi(E_T) - \int_{t}^{T}\left(Z_s \textrm{  }0 \right)\ud W_s
\end{align*}

Where the $W_s$ is a 2-dim Brownian motion.
Hence the algorithm becomes:
\begin{itemize}
\item $\forall x \in C_N, \bar{u}(T,x) = \phi(x)$.
\item $\forall k\in\{0,...,N-1\}, \forall x\in C_k$
\begin{align*}
&T(t_k,x) = \left(\begin{array}{c}
		0\\
		p-\bar{u}(t_{k+1},x)
	\end{array}\right)h + \left(\begin{array}{c}
		\sigma g(\Delta W^k) \\
		0 
	\end{array}\right)\\
&\bar{u}(t_{k},x) = \mathbb{E}[\bar{u}(t_{k+1},\Pi(x+T(t_k,x)))]
\end{align*}

\end{itemize}

Where $x = (p,e)$ and $g(\Delta B^k)$ denotes the quantization of brownian motion of dimension 1, since the second component of 2-dim brownian motion does not play a role in the algorithm, so we only need to simulate the first component.

For implementations of Menozzi-Delaure method, we use number of time steps = 80 and also number of space steps = 150 for different volatility in the price process $P_t$.
We observe that for $\sigma$ large enough, Menozzi's method works well however when $\sigma$ decreases, this method gives an inconsistent result which is not what we want. So we need to find an another method which should be valid for all cases: non-vanishing and vanishing case.

%\begin{figure}[ht]
%\begin{minipage}{0.3\linewidth}
%%\centering  % redundant
%\includegraphics[width=\textwidth]{delaure_1.png}
%\caption{$\sigma=1$}
%\label{fig:figure1}
%\end{minipage}%
%\hfill% not: "\hspace{0.5cm}"
%\begin{minipage}{0.3\linewidth}
%%\centering  % redundant
%\includegraphics[width=\textwidth]{delarue_02.png}
%\caption{$\sigma=0.3$}
%\label{fig:figure2}
%\end{minipage}%
%\hfill% not: "\hspace{0.5cm}"
%\begin{minipage}{0.3\linewidth}
%%\centering  % redundant
%\includegraphics[width=\textwidth]{delaure_001.png}
%\caption{$\sigma=0.01$}
%\label{fig:figure3}
%\end{minipage}
%\end{figure}
